# Supplementary material for: Continuous Object Representation Networks: Novel View Synthesis without Target View Supervision
Source: arXiv:2007.15627 source file (2020-10-23)

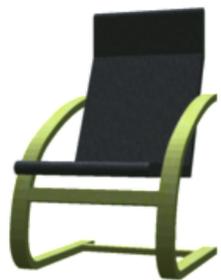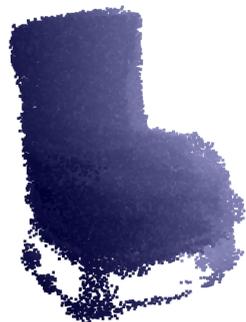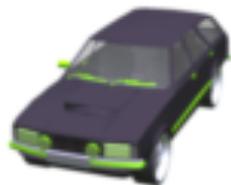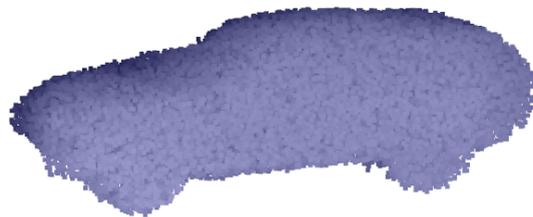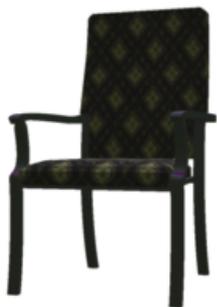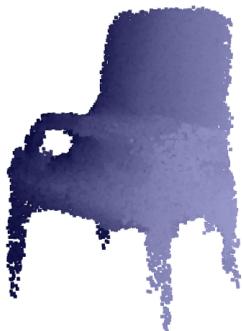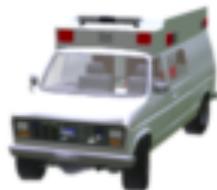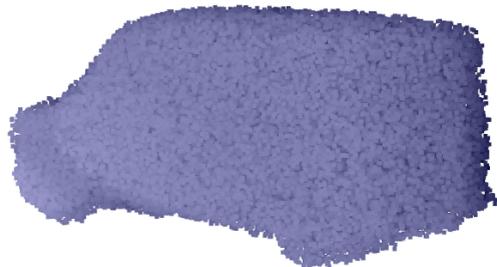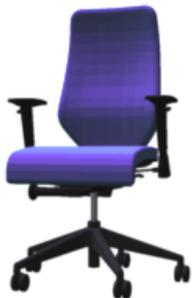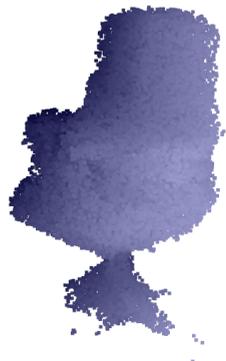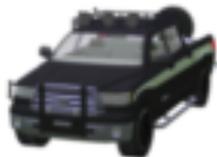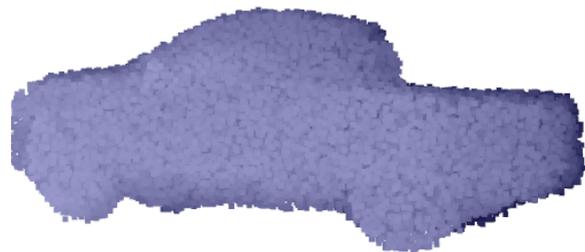

Supplement: Supplementary file 2 [file supp_recon3d.pdf]
